# Supplementary material for: Few-Body Quantum Chaos, Localization, and Multi-Photon Entanglement in Optical Synthetic Frequency Dimension
Source: arXiv:2406.07346 source file (2024-06-11)

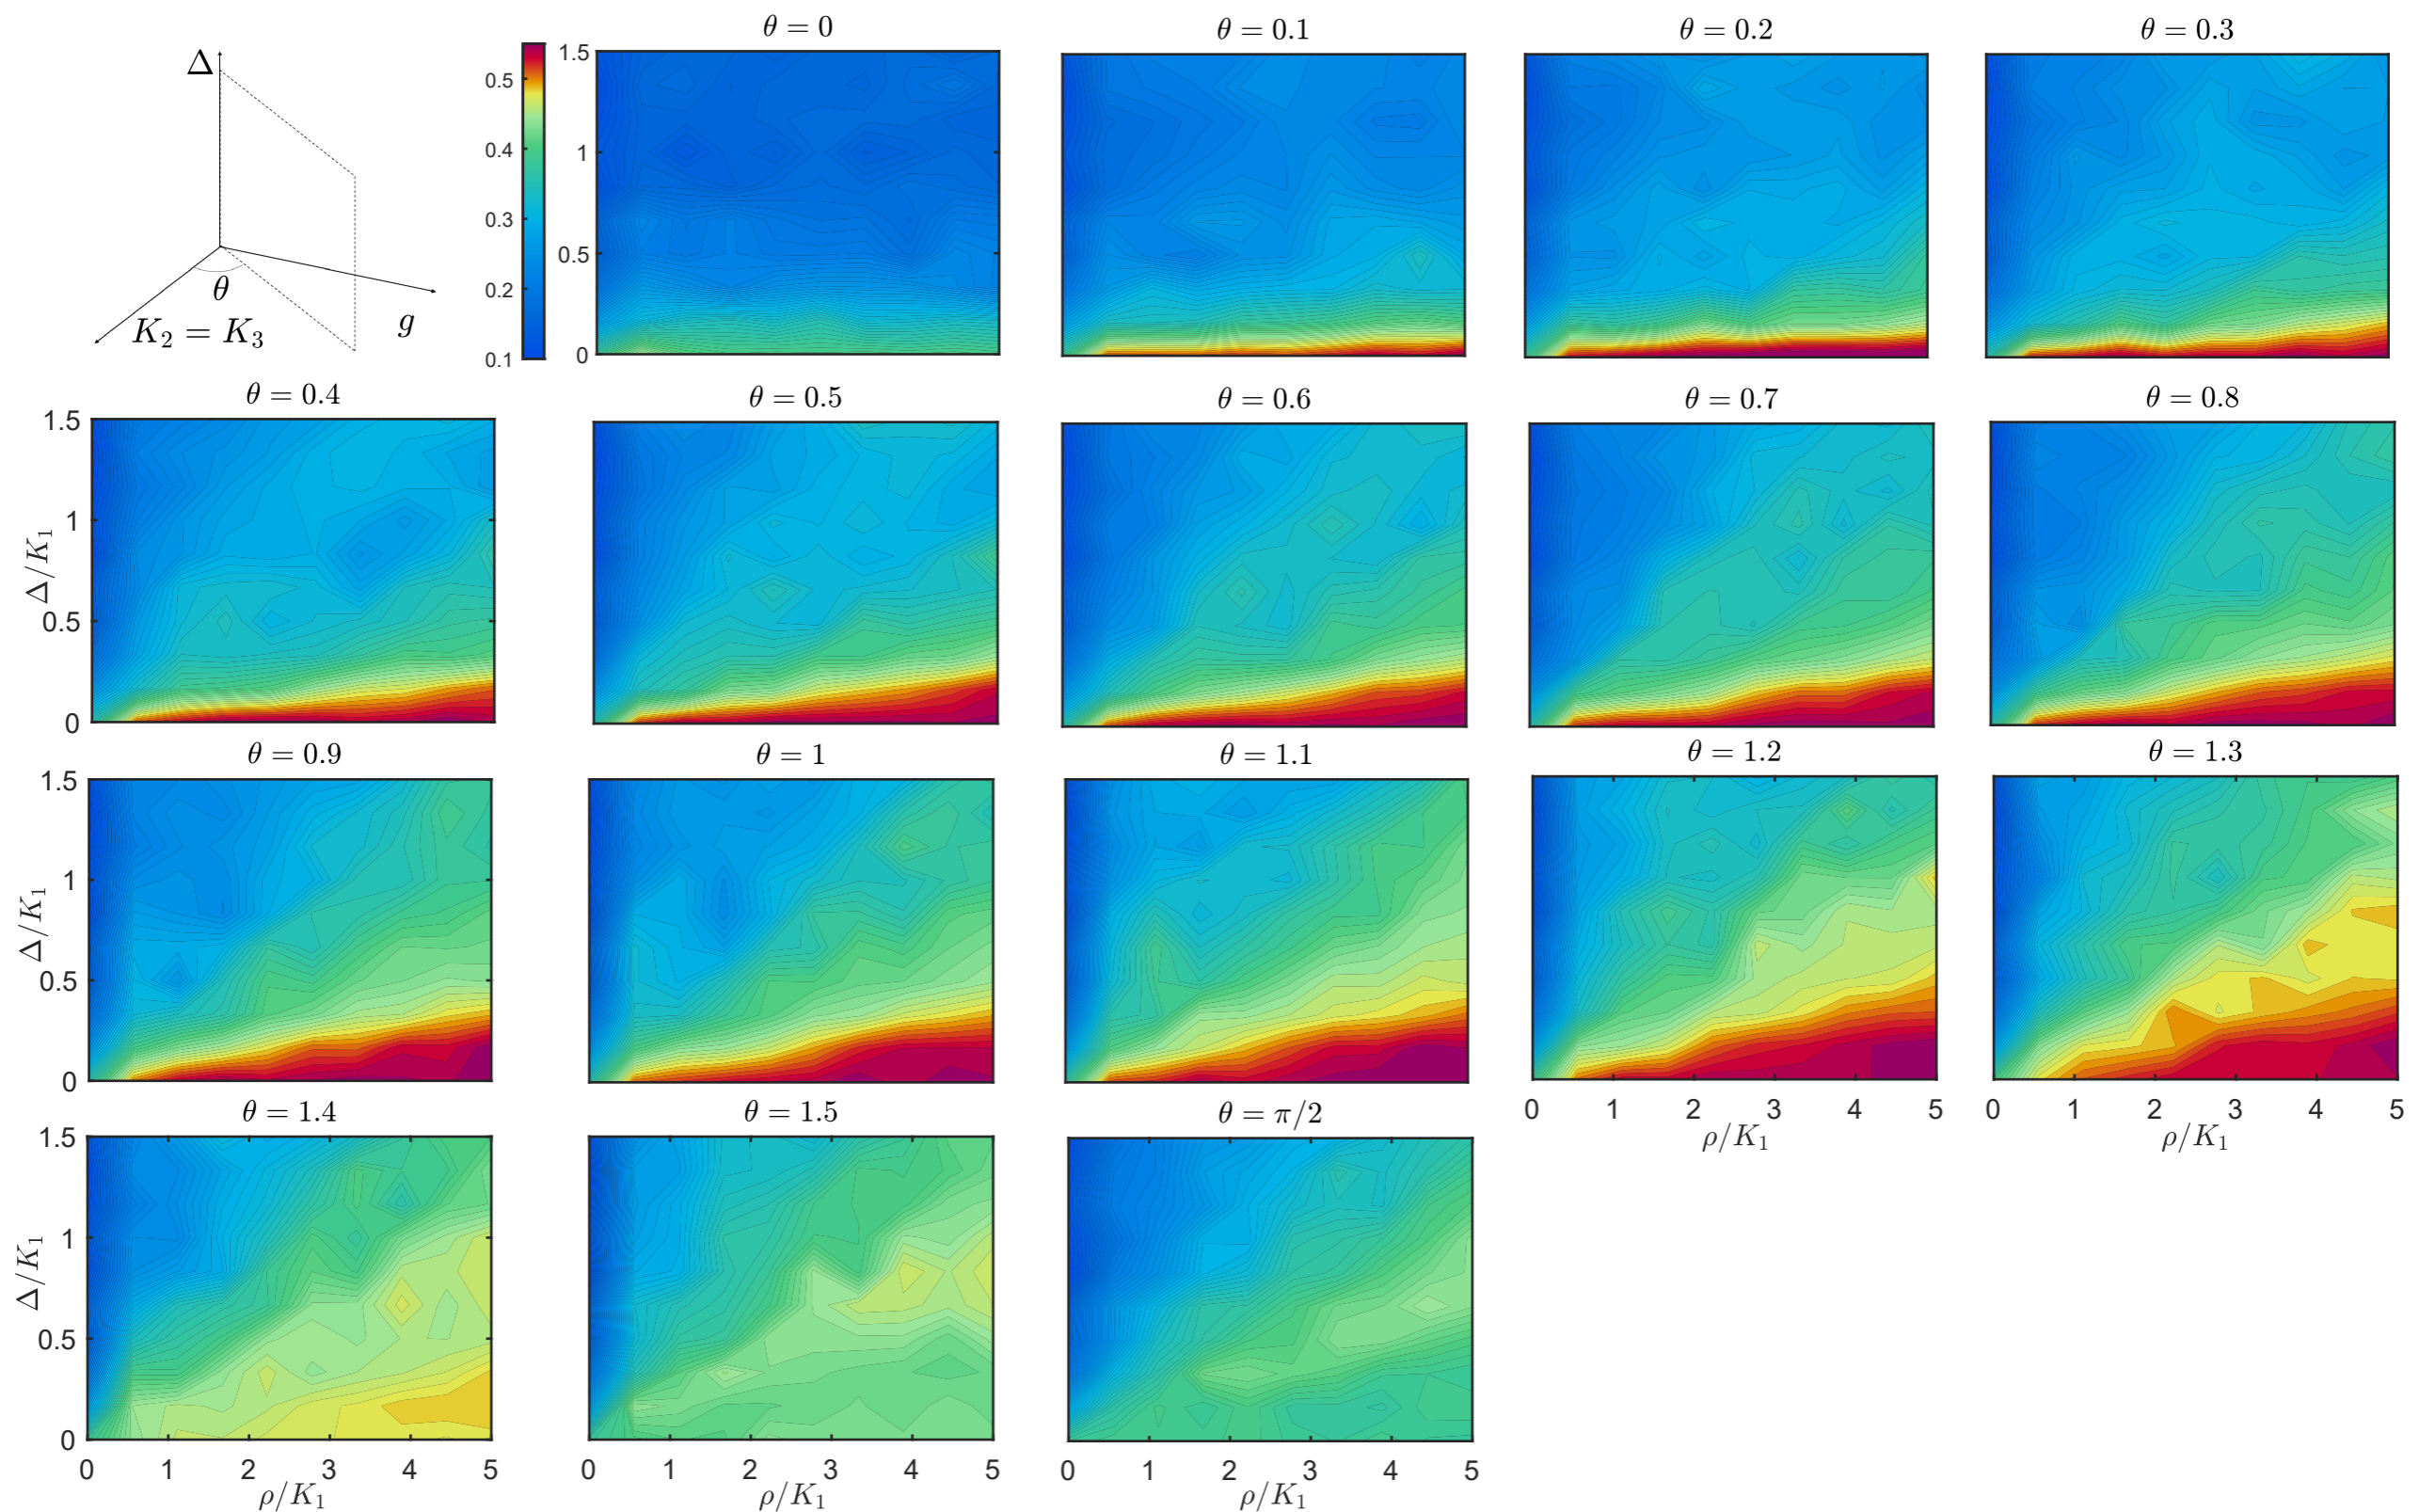

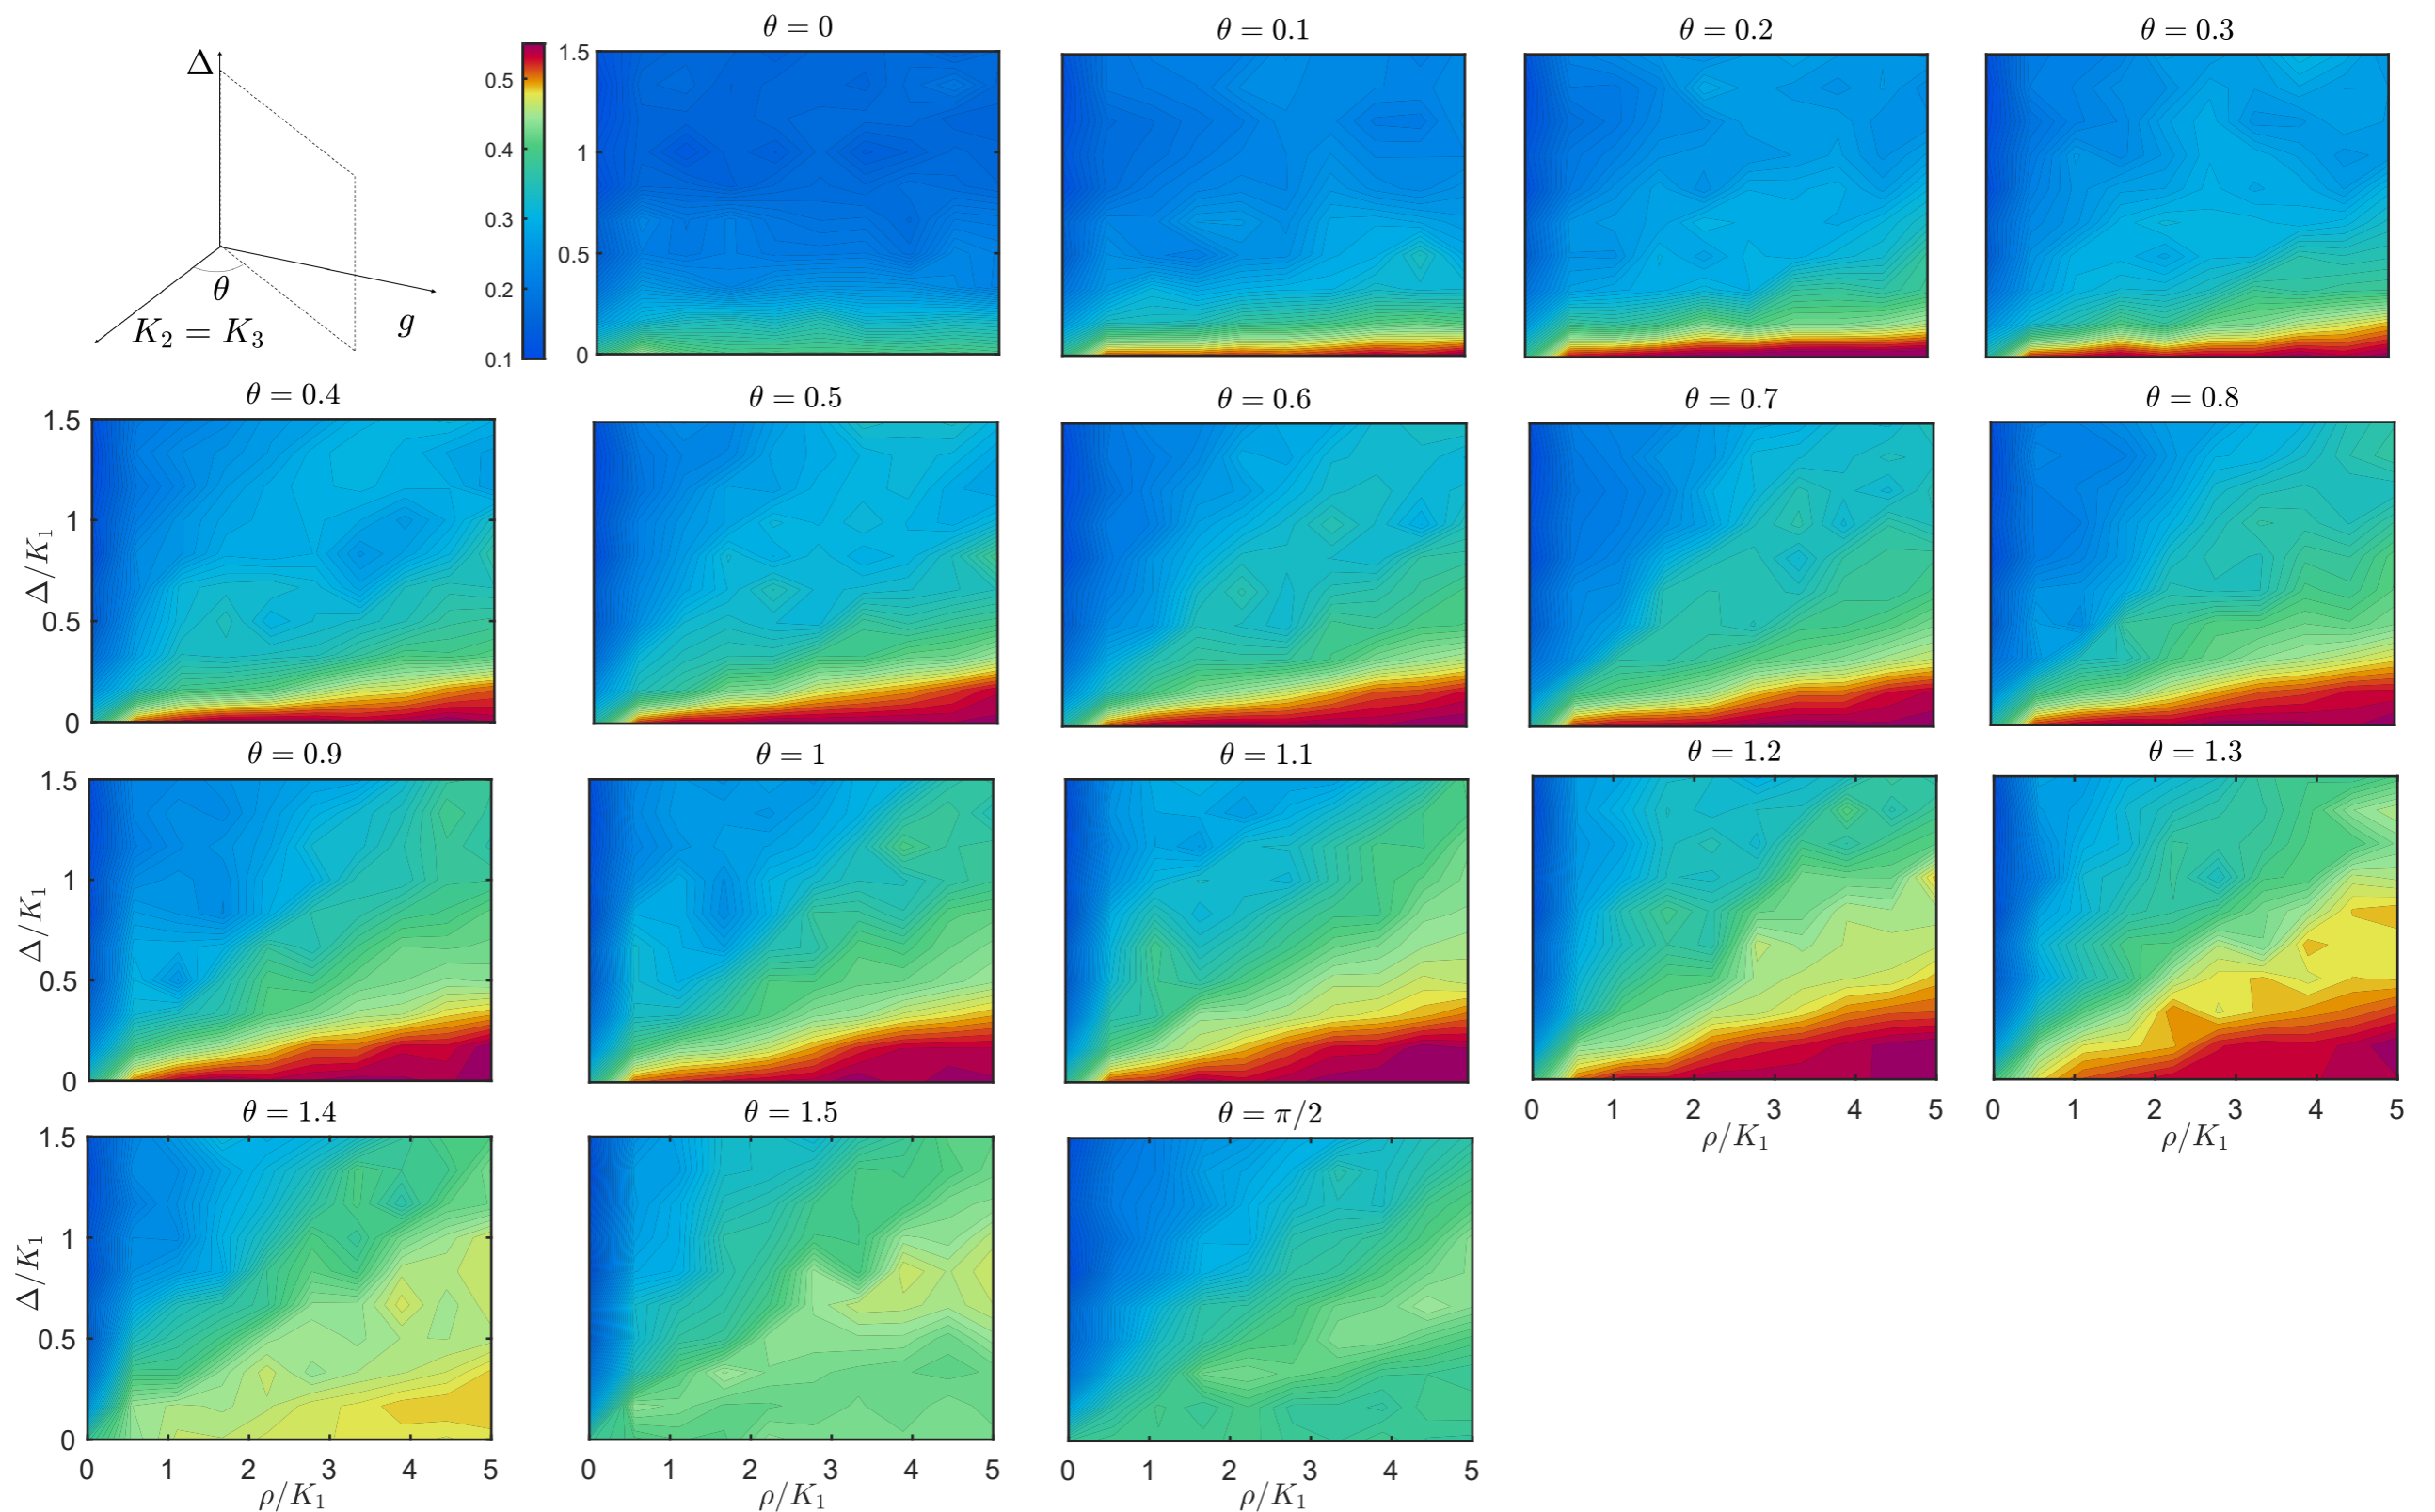

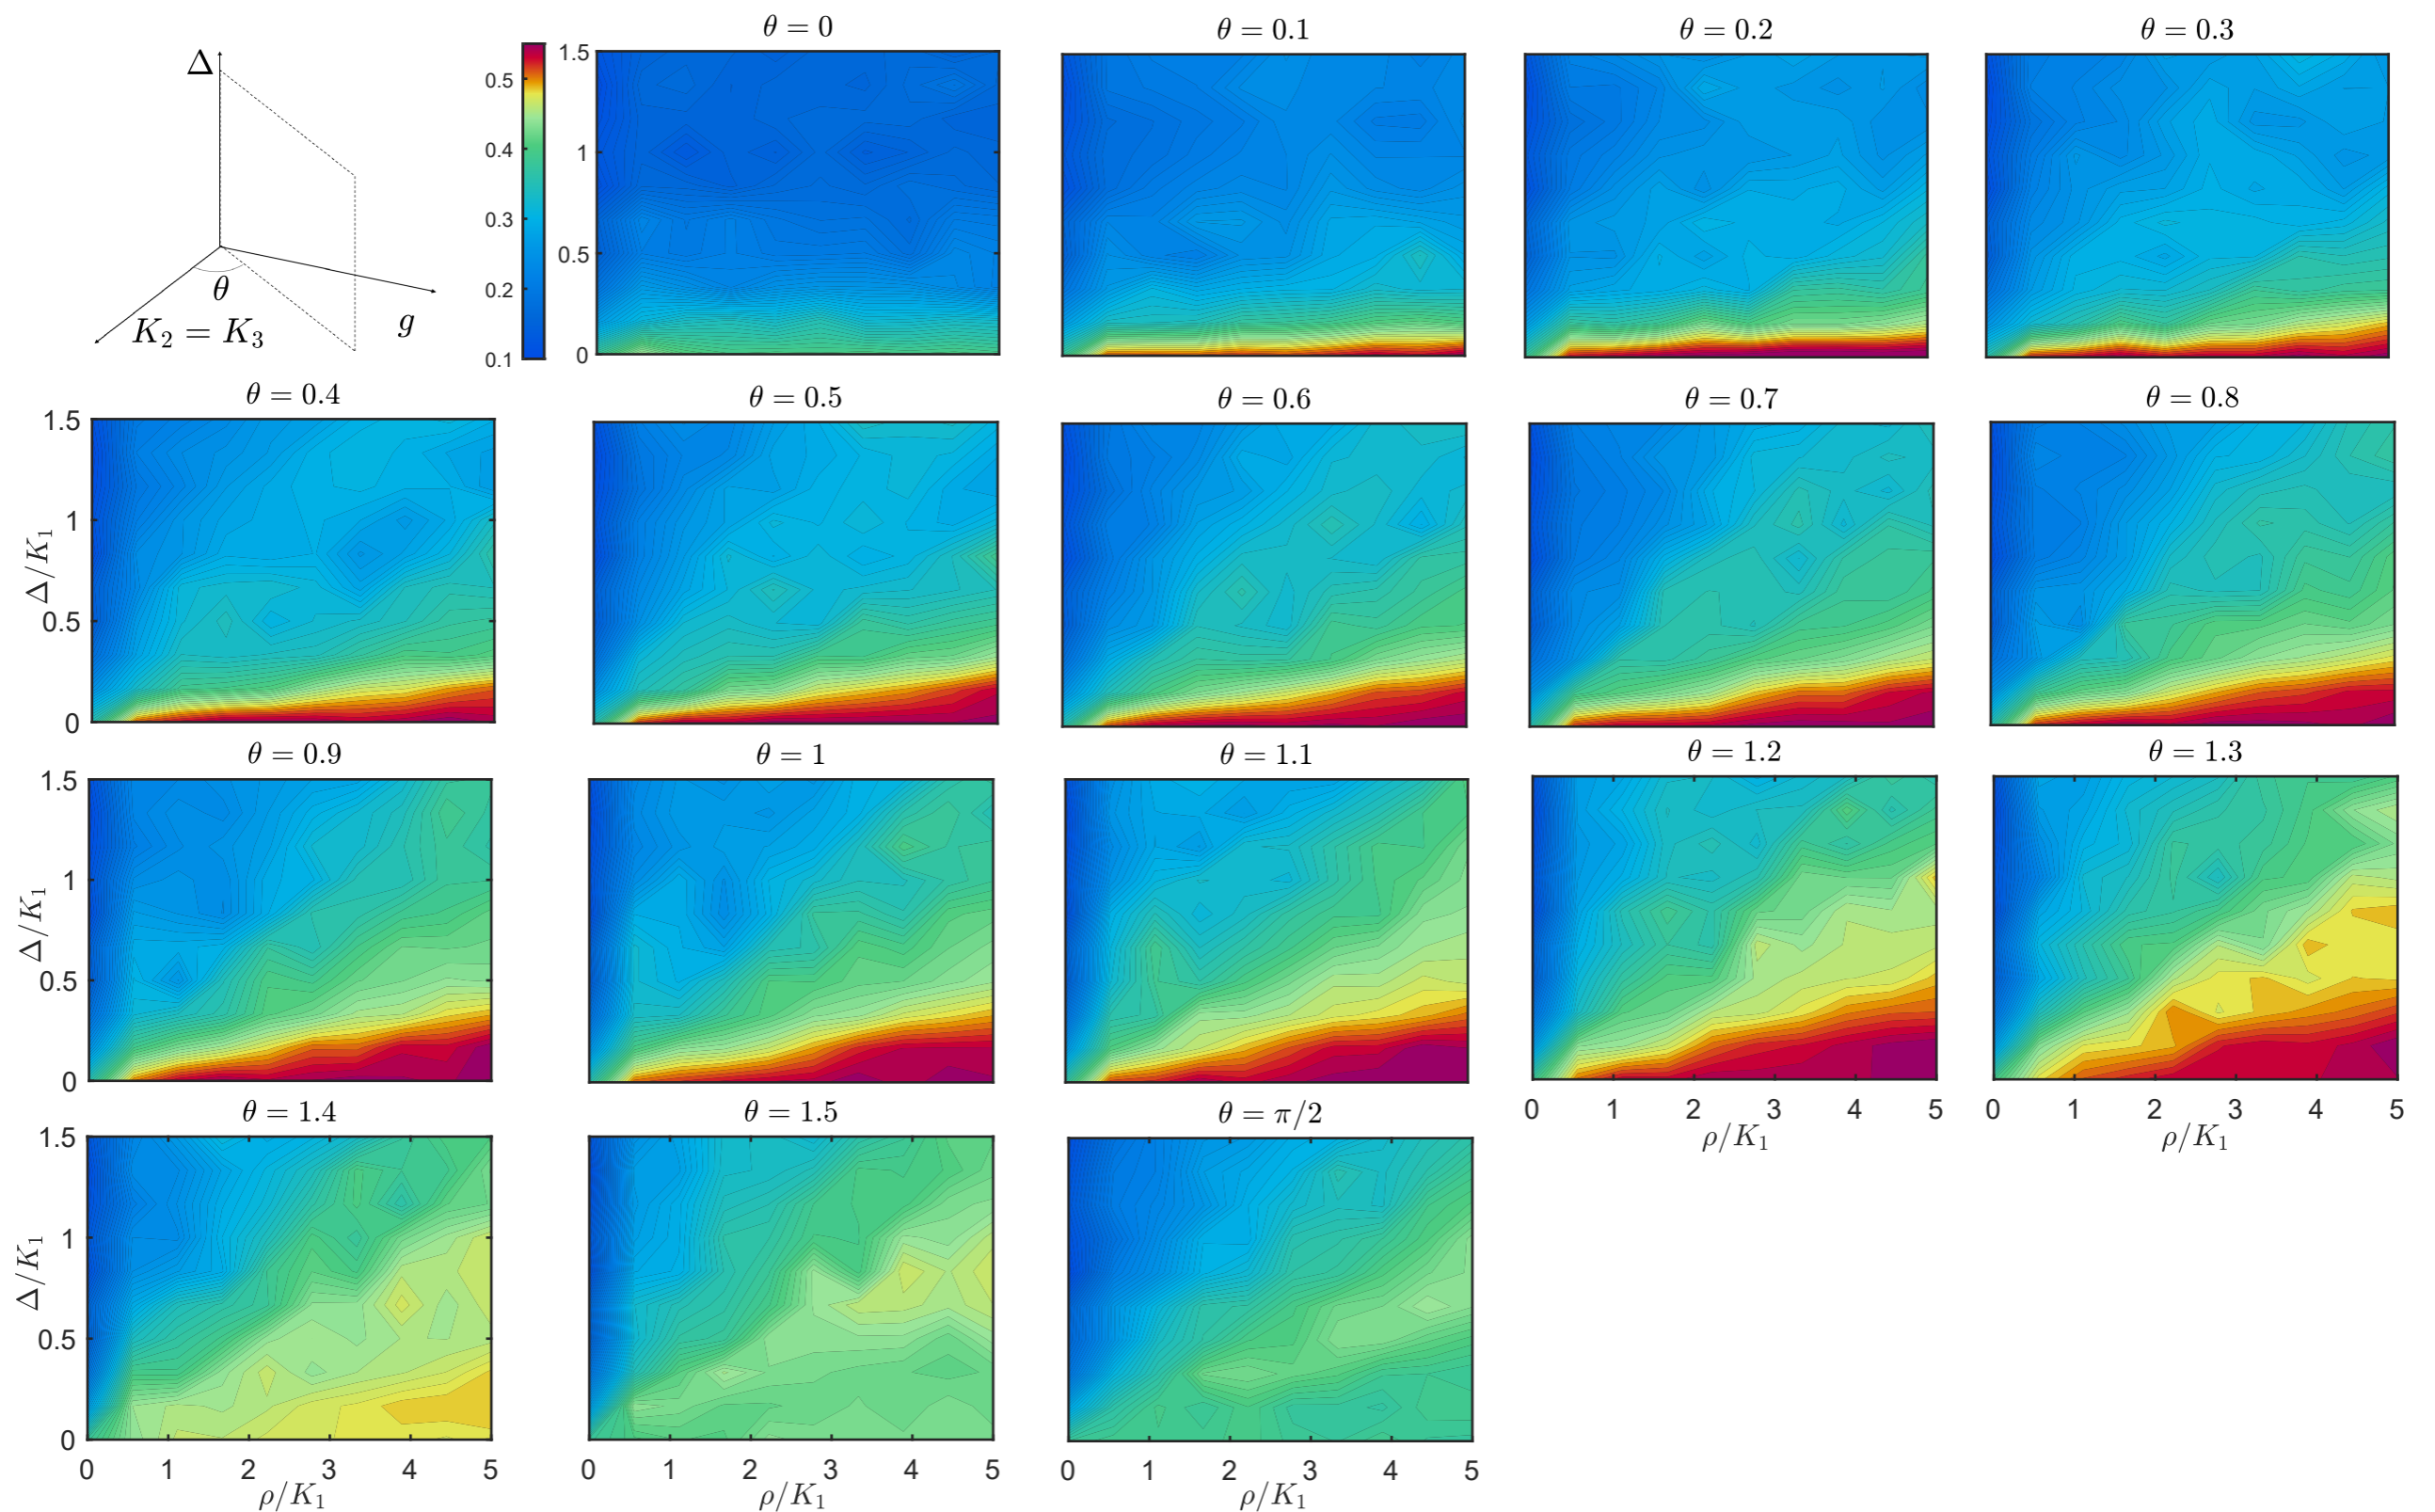

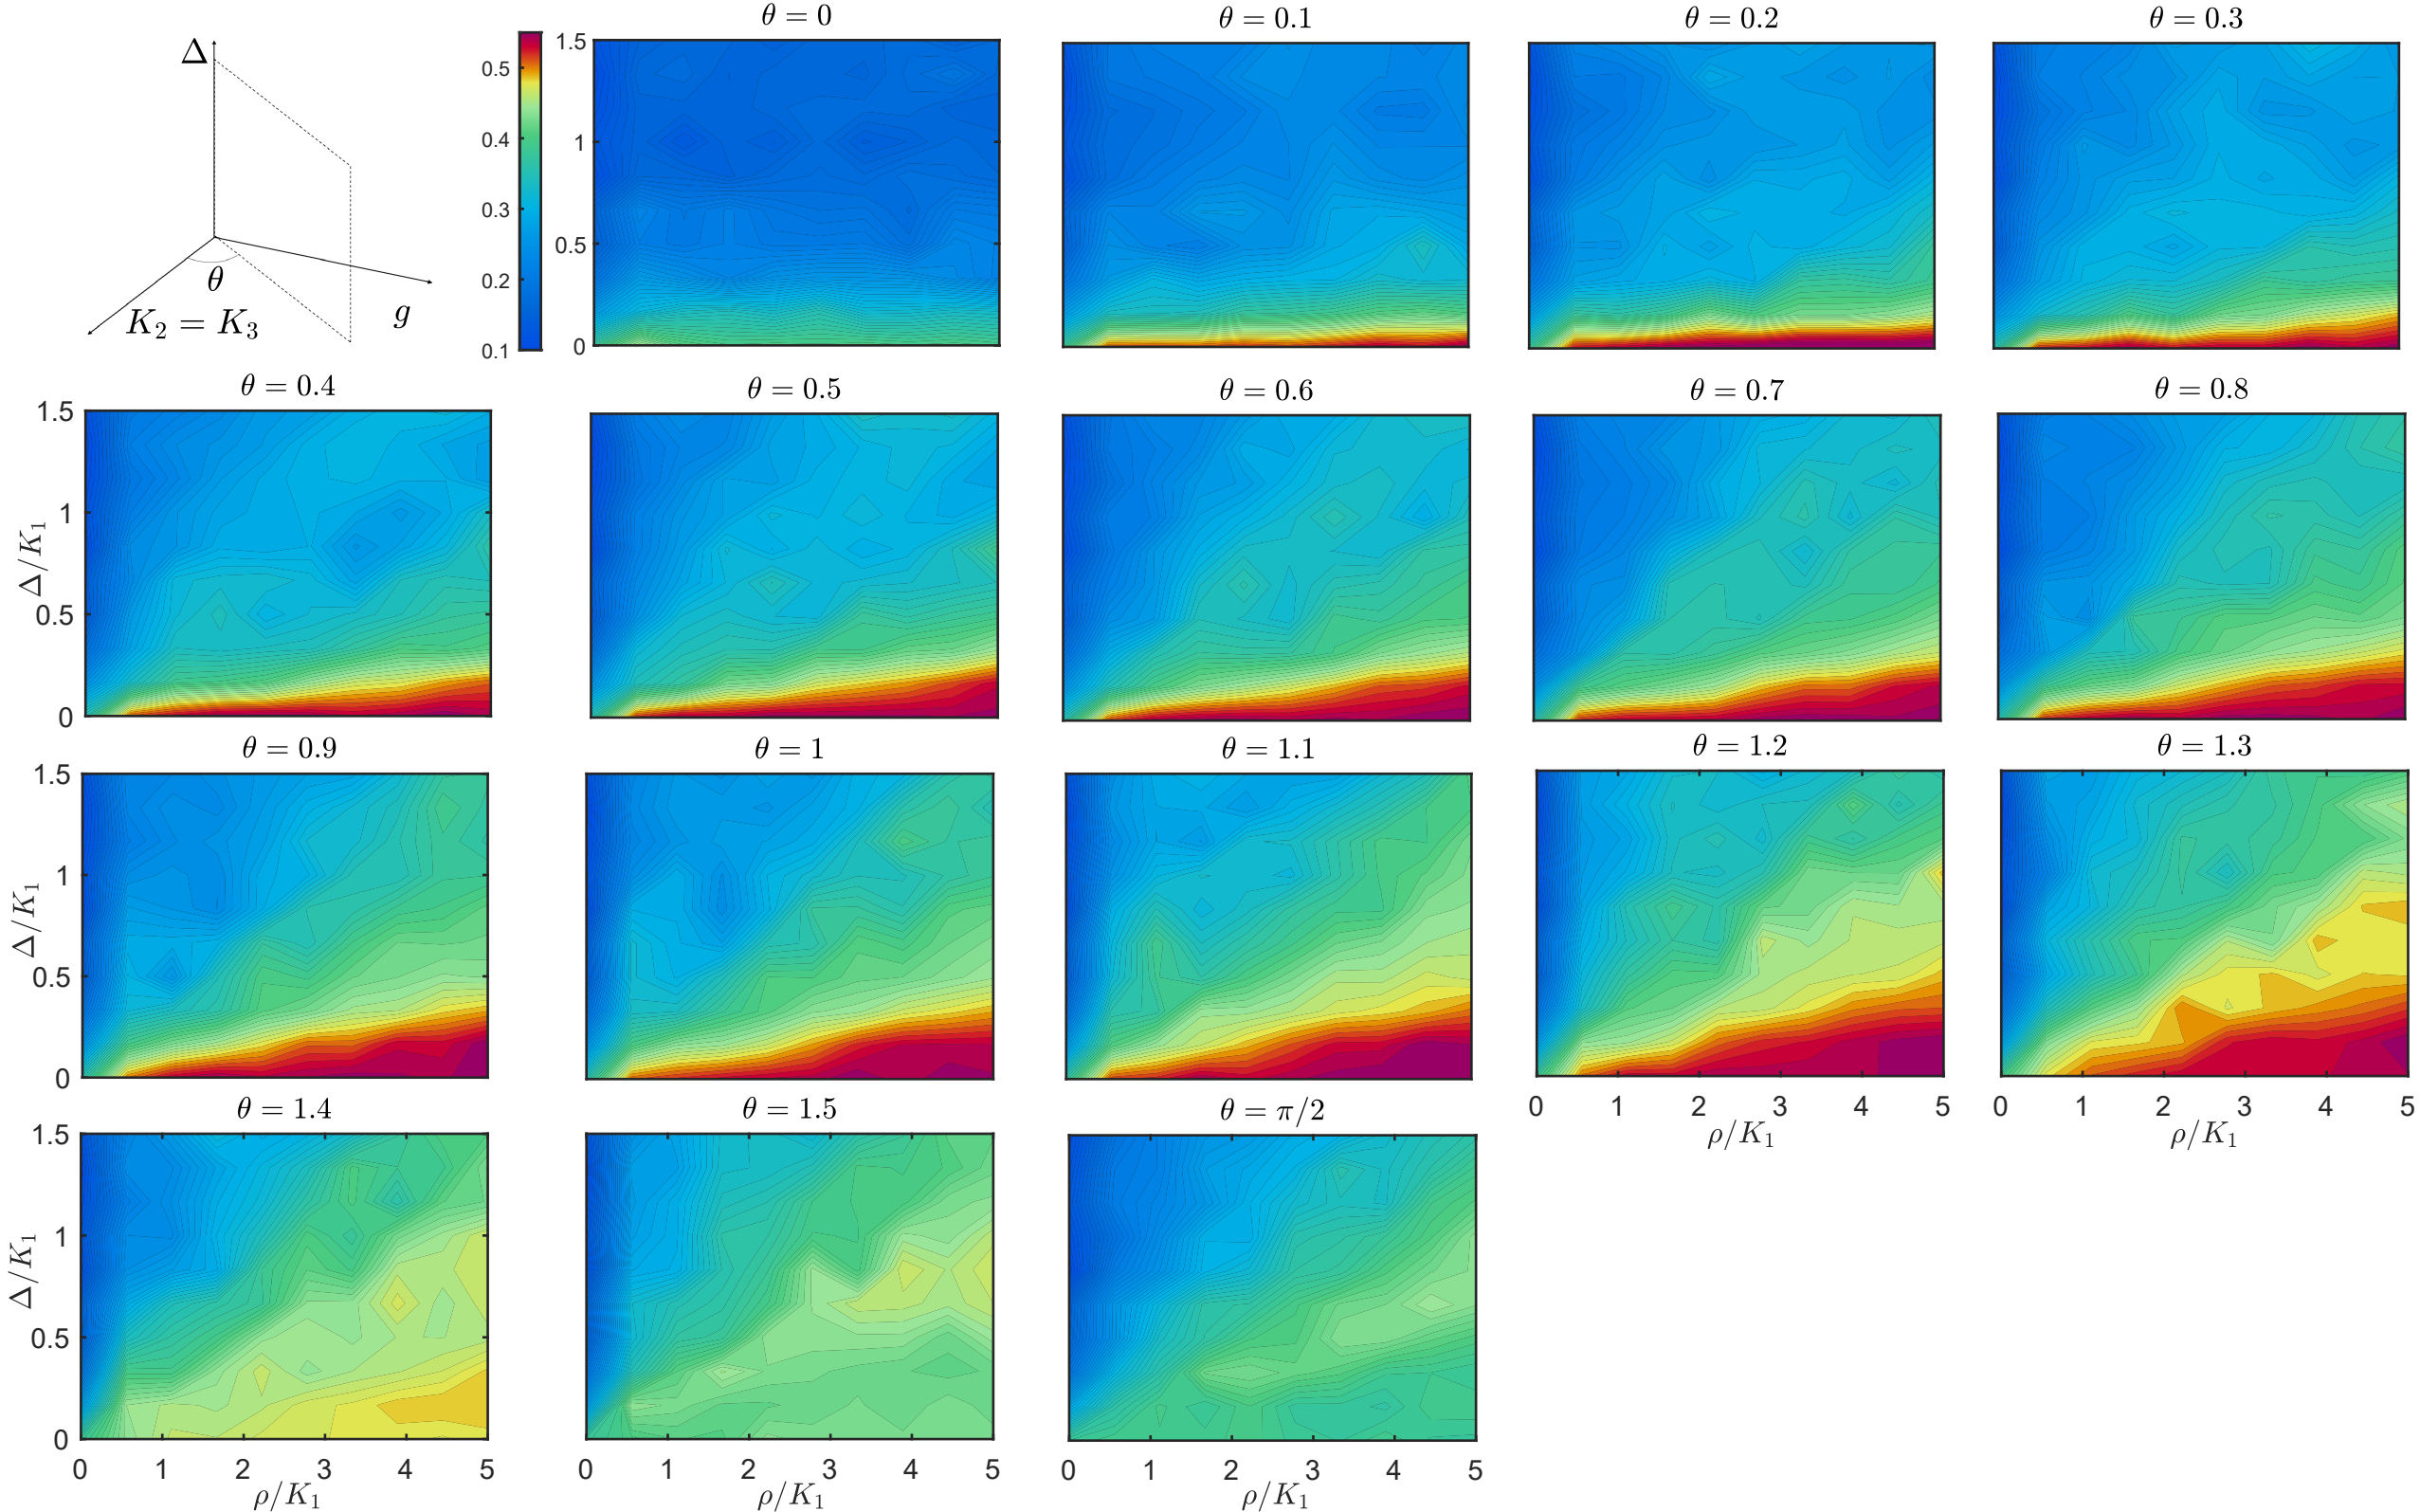

Supplement: Supplementary file 1 [file SM_phase.pdf]
